# Supplementary material for: Impact of tidal environment on galaxy clustering in GAMA
Source: arXiv:2305.01266 source file (2023-12-05)
Supplement: Supplementary file 1 [file appendix.tex]

\appendix

\section{Parameter-dependent covariance matrix}
\AP{To do: (i) Measure mean and error of each element of correlation matrix and ask how statistically different are the original and best fit matrices. (ii) Test eigenspace structure of subset of data covariance (e.g. $\xi_4$ measurements) as well as full covariance. (iii) Is there a rotation of data that minimises the effects of parameter dependence in covariannce matrix? \red{(explored below)} (iv) Fisher analysis using $\nabla\Cal{C}$ measurements (for followup project).}

We collect here some results related to parameter dependent covariance matrices.
In the following, the data are assumed to be $N_{\rm d}$-dimensional, indexed by Greek indices $1\leq \alpha,\beta,\ldots\leq N_{\rm d}$, and the model has $N_{\rm m}$ parameters, indexed by Latin indices $1\leq i,j,\ldots\leq N_{\rm m}$. 

\subsection{General results}
We start by closely following the discussion in section 3.2 of \citet{heavens09}, generalising those results (which are presented for Gaussian-distributed data) to an arbitrary distribution of the data.

Let $d$ be the $N_{\rm d}$-dimensional data vector, drawn from a distribution $\Cal{P}$ with mean $\mu_0$, covariance $\Cal{C}_0$ and unspecified higher cumulants:
\be
d\sim \Cal{P}(\mu_0,\Cal{C}_0,\ldots)\,.
\label{app:datadist}
\ee
If the third and higher cumulants all vanish, then the data are Gaussian distributed, but we will not make this assumption below.
The model with parameter vector $\theta$ defines a parameter-dependent mean vector $\mu(\theta)$ and parameter-dependent covariance matrix $\Cal{C}(\theta)$. 
The subscript $0$ in \eqn{app:datadist} refers to the `true' model parameters $\theta_0$ and reminds us that the statistical properties of the data are determined by the true parameter values: $\mu_0=\mu(\theta_0)$ and $\Cal{C}_0=\Cal{C}(\theta_0)$.

The mean $\mu(\theta)$ and covariance $\Cal{C}(\theta)$ can be used to construct the Fisher information matrix as follows. For brevity, we will henceforth drop the explicit parameter dependence in $\mu$ and $\Cal{C}$. First consider the parameter-dependent quadratic quantity $\Cal{D}$ defined as
\be 
\Cal{D} \equiv \left(d - \mu\right)\,\left(d - \mu\right)^{\rm T}\,,
\label{app:D-def}
\ee
where the superscript `T' indicates a transpose.
Differentiating $\Cal{D}$ with respect to the parameters (using $\nabla_i\equiv\p/\p\theta^i$) and taking expectation values using the distribution in \eqn{app:datadist} gives us the following relations
\begin{align}
\avg{\Cal{D}} &= \Cal{C}_0 + \left(\mu-\mu_0\right)\,\left(\mu-\mu_0\right)^{\rm T}\,,
\label{app:<D>}\\
\avg{\nabla\Cal{D}} &= \nabla\mu \left(\mu-\mu_0\right)^{\rm T} + \left(\mu-\mu_0\right) \nabla\mu^{\rm T}\,,
\label{app:<dD>}\\
\avg{\nabla\nabla\Cal{D}} &= 2\left(\nabla\mu\nabla\mu^{\rm T}\right) \notag\\
&\ph{2()}
+ \nabla\nabla\mu \left(\mu-\mu_0\right)^{\rm T} + \left(\mu-\mu_0\right) \nabla\nabla\mu^{\rm T}\,,
\label{app:<ddD>}
\end{align}
where the parentheses in the first term of the last equation indicate symmetrisation.

Next, note that the quantity $\chi^2$ (or $-2$ times the log-likelihood) minimised in MCMC algorithms typically follows from writing a Gaussian-shaped likelihood for the data vector and can be reduced to the form
\be 
\chi^2 = {\rm Tr}\left[\ln\Cal{C} + \Cal{C}^{-1}\Cal{D}\right]\,,
\label{app:chi2}
\ee 
where `Tr' stands for the trace, and we used the determinant identity $\ln({\rm det}\Cal{C}) = {\rm Tr}\ln\Cal{C}$. The derivatives of $\chi^2$ can be simplified using the identities $\nabla\ln\Cal{C}=\Cal{C}^{-1}\nabla\Cal{C}$ and $\nabla\left(\Cal{C}^{-1}\right)=-\Cal{C}^{-1}\nabla\Cal{C}\,\Cal{C}^{-1}$ to give
\begin{align}
\nabla\chi^2 &= {\rm Tr} \left[\Cal{C}^{-1}\nabla\Cal{C}\left(\mathbb{1}-\Cal{C}^{-1}\Cal{D}\right) + \Cal{C}^{-1}\nabla\Cal{D}\right]\,,
\notag\\
\nabla\nabla\chi^2 &= {\rm Tr} \left[\Cal{C}^{-1}\nabla\nabla\Cal{C}\left(\mathbb{1}-\Cal{C}^{-1}\Cal{D}\right)\right. \notag\\
&\ph{{\rm Tr}\left[\Cal{C}^{-1}\right]}
- \Cal{C}^{-1}\nabla\Cal{C}\,\Cal{C}^{-1}\nabla\Cal{C}\left(\mathbb{1}-2\,\Cal{C}^{-1}\Cal{D}\right) \notag\\
&\ph{{\rm Tr}\left[\Cal{C}^{-1}-\right]}
\left.- 2\,\Cal{C}^{-1}\nabla\Cal{C}\,\Cal{C}^{-1}\nabla\Cal{D}
+ \Cal{C}^{-1}\nabla\nabla\Cal{D}\right]\,,
\label{app:dchi2:ddchi2}
\end{align}
where $\mathbb{1}$ is the $N_{\rm d}$-dimensional identity matrix. Taking expectation values, using \eqns{app:<D>}-\eqref{app:<ddD>} and simplifying, we get
\begin{align}
&\avg{\nabla\chi^2} \notag\\
&= {\rm Tr}\left[\Cal{C}^{-1}\nabla\Cal{C}\left(\mathbb{1}-\Cal{C}^{-1}\Cal{C}_0 - \Cal{C}^{-1}(\mu-\mu_0)(\mu-\mu_0)^{\rm T}\right) \right. \notag\\
&\ph{{\rm Tr}\left[\Cal{C}^{-1}\right]}
+ \left.\Cal{C}^{-1}\left(\nabla\mu\,(\mu-\mu_0)^{\rm T} + (\mu-\mu_0)\nabla\mu^{\rm T}\right)\right]\,,
\label{app:<dchi2>}\\
&\avg{\nabla\nabla\chi^2} \notag\\
&= {\rm Tr}\left[\Cal{C}^{-1}\nabla\nabla\Cal{C}\left(\mathbb{1}-\Cal{C}^{-1}\Cal{C}_0 - \Cal{C}^{-1}(\mu-\mu_0)(\mu-\mu_0)^{\rm T}\right)\right. \notag\\
&
- \Cal{C}^{-1}\nabla\Cal{C}\,\Cal{C}^{-1}\nabla\Cal{C}\left(\mathbb{1}-2\Cal{C}^{-1}\Cal{C}_0 - 2\Cal{C}^{-1}(\mu-\mu_0)(\mu-\mu_0)^{\rm T}\right) \notag\\
&
- 2\,\Cal{C}^{-1}\nabla\Cal{C}\,\Cal{C}^{-1}\left(\nabla\mu\,(\mu-\mu_0)^{\rm T} + (\mu-\mu_0)\nabla\mu^{\rm T}\right) \notag\\
&
+ \left.\Cal{C}^{-1}\left( 
\nabla\nabla\mu \left(\mu-\mu_0\right)^{\rm T} + \left(\mu-\mu_0\right) \nabla\nabla\mu^{\rm T} + 2\left(\nabla\mu\nabla\mu^{\rm T}\right)\right)\right]\,,
\label{app:<ddchi2>}
\end{align}
It will be useful below to define a generalised $N_{\rm m}\times N_{\rm m}$ Fisher information matrix \Cal{F}\ by
\be 
\Cal{F} \equiv \frac12\,\avg{\nabla\nabla\chi^2}\,.
\label{app:Fisher-def}
\ee
Equations~\eqref{app:<dchi2>} and~\eqref{app:<ddchi2>} hold for generically distributed data when the likelihood is assumed to have a Gaussian shape. We are interested in the following special cases of this general result.

\subsubsection{Fully parameter-dependent moments} 
If the full parameter dependence of $\mu$ and $\Cal{C}$ is accounted for, then it is clear that evaluating \eqn{app:<dchi2>} at $\theta=\theta_0$ leads to $\avg{\nabla\chi^2}=0$, with both lines on the right hand side independently vanishing. 
Thus, on average, the likelihood is extremised at the true parameter values.
In this case, from \eqn{app:<ddchi2>} one also recovers the usual definition of the Fisher matrix $\Cal{F}_0$ (which assumes evaluation at $\theta=\theta_0$) as
\be
\Cal{F}_0 = {\rm Tr}\left[\frac12\Cal{C}_0^{-1}\nabla\Cal{C}_0\,\Cal{C}_0^{-1}\nabla\Cal{C}_0 + \Cal{C}^{-1}_0\left(\nabla\mu_0\nabla\mu_0^{\rm T}\right)\right]\,,
\label{app:F0}
\ee
which is consistent with, e.g., equation~(62) of \citet{heavens09}. Thus, when accounting for the full parameter dependence of the mean and covariance of the model prediction, the maximum likelihood estimate of parameters is statistically unbiased and leads to parameter errors given by the inverse of $\Cal{F}_0$.

\subsubsection{Fixed covariance} 
Suppose we ignore the parameter dependence of the covariance matrix \Cal{C}\ and instead \emph{fix its value} to that at some fiducial choice of parameters $\theta=\theta_{\rm fid}\neq\theta_0$, such that $\Cal{C}=\Cal{C}(\theta_{\rm fid}) \equiv \Cal{C}_{\rm fid}$ and $\nabla\Cal{C}=0=\nabla\nabla\Cal{C}$. The mean $\mu$ on the other hand is assumed to depend on the parameters as usual. This is a common approximation in many cosmological large-scale structure analyses.

Interestingly, since the first term in \eqn{app:<dchi2>} involves $\nabla\Cal{C}$ which is now assumed to vanish, we again have $\avg{\nabla\chi^2}=0$ at $\mu=\mu_0$, i.e., $\theta=\theta_0$. In other words, despite ignoring the parameter-dependence of \Cal{C}, the maximum likelihood estimator of $\theta$ is still statistically unbiased. However, since we are no longer accounting for the variation of \Cal{C} with $\theta$, in this case the expression of the Fisher information matrix (evaluated at $\theta=\theta_0$) changes from $\Cal{F}_0$ to $\Cal{F}_{\rm fid}$ given by
\be 
\Cal{F}_{\rm fid} = {\rm Tr}\left[\Cal{C}^{-1}_{\rm fid}\left(\nabla\mu_0\nabla\mu_0^{\rm T}\right)\right]\,,
\label{app:Ffid}
\ee
which differs from $\Cal{F}_0$ (equation~\ref{app:F0}) through the absence of the term involving $\nabla\Cal{C}_0$ and the replacement $\Cal{C}_0\to\Cal{C}_{\rm fid}$ in the term involving derivatives of $\mu$.

Thus, using a fixed covariance matrix is unlikely to bias the estimate of the true parameter values, provided the Gaussian-shaped likelihood is a reasonable description of the actual distribution of the data. The parameter errors, however, can be affected by this choice. In the case where some parameter is assumed to have fiducial value zero but actually has a non-zero true value, the detection significance of that parameter could be mis-estimated as a result of incorrectly assuming a fixed data covariance. Whether this is an over-estimate or under-estimate will depend on the specific data set and model being considered. 

If the maximum likelihood estimate of parameters for a given data set is denoted $\hat\theta$ (so that $\avg{\hat\theta}=\theta_0$), then we can define the `detection significance' of the measurement of the $i^{\rm th}$ parameter as the error-weighted difference between $\hat\theta_i$ and the fiducial parameter value $\theta_{{\rm fid},i}$. This way of thinking is particularly meaningful for those parameters whose fiducial value is zero, such as assembly bias parameters. Since the marginal error on $\theta_i$ is $\sqrt{(\Cal{F}^{-1})_{ii}}$, the detection significance $S_{0,i}$ accounting for the full parameter-dependence of $\Cal{C}$ is
\be 
S_{0,i} = \left(\hat\theta_i-\theta_{{\rm fid},i}\right)/\sqrt{(\Cal{F}^{-1}_{0})_{ii}}\,,
\label{app:S0}
\ee
while the (incorrect) detection significance $S_{{\rm fid},i}$ assuming $\Cal{C}=\Cal{C_{\rm fid}}$ is
\be 
S_{{\rm fid},i} = \left(\hat\theta_i-\theta_{{\rm fid},i}\right)/\sqrt{(\Cal{F}^{-1}_{\rm fid})_{ii}}\,,
\label{app:Sfid}
\ee
where $\Cal{F}_0$ and $\Cal{F}_{\rm fid}$ were respectively given by \eqns{app:F0} and~\eqref{app:Ffid}. 

In practice, if parameter estimation has been performed assuming $\Cal{C}=\Cal{C}_{\rm fid}$, then instead of quoting the detection significance from \eqn{app:Sfid}, it would be more accurate to quote \eqn{app:S0}, with $\Cal{F}_0$ being estimated using \eqn{app:F0} evaluated at $\theta=\hat\theta$. \AP{shadab, do you agree?}

\subsection{Perturbative results}
If we assume that the parameter dependence is weak in the vicinity of the fiducial parameters $\theta_0$, so that
\begin{align}
\Cal{C}(\theta) &= \Cal{C}(\theta_0) + \left(\theta-\theta_0\right) \cdot \nabla \Cal{C} + \ldots \notag\\
&\equiv \Cal{C}_0 + \delta\theta \cdot \nabla \Cal{C} + \ldots\,,
\label{app:C(theta)}
\end{align}
where $\Cal{C}_0$ is the data covariance evaluated at the fiducial parameters and $\nabla\Cal{C}$ is the derivative of the data covariance with respect to the parameters, also evaluated at the fiducial parameters: $(\nabla\Cal{C})_i = \p\Cal{C}/\p\theta_i|_{\theta=\theta_0}$, and we defined $\delta\theta \equiv \theta-\theta_0$.

We are interested in the behaviour of the inverse covariance $\Cal{C}^{-1}(\theta)$ which appears in the log-likelihood as in \eqn{app:loglike}. Keeping lowest order terms in $\delta\theta\cdot\nabla\Cal{C}$, we have
\be 
\Cal{C}^{-1}(\theta) = \Cal{C}_0^{-1} - \Cal{C}_0^{-1}\left(\delta\theta\cdot\nabla\Cal{C}\right)\Cal{C}_0^{-1} + \ldots\,.
\label{app:Cinv}
\ee 
Since $\Cal{C}_0^{-1}$ is real and positive semi-definite, it can be diagonalised by an $N_{\rm d}$-dimensional rotation $R_0$:
\be 
R_0^{\rm T}\,\Cal{C}_0^{-1}\, R_0 = \Lambda_0\,,
\label{app:diagC0inv}
\ee 
where $(\Lambda_0)_{\alpha\beta} = \lambda_{0\alpha}\delta_{\alpha\beta}$.

Let $R$ be the rotation that diagonalises $\Cal{C}^{-1}$. Since $\Cal{C}^{-1}$ and $\Cal{C}_0^{-1}$ are close to each other, we can expect $R = R_0(\mathbf{1}+\epsilon)$ where $\epsilon$ is of the same parametric order as $\delta\theta\cdot\nabla\Cal{C}$. The condition $R^{\rm T}=R^{-1}$ at leading order in $\epsilon$ implies that $\epsilon$ must be antisymmetric ($\epsilon^{\rm T}=-\epsilon$) as expected from the generator of an infinitesimal rotation. Straightforward algebra then gives
\be 
\Lambda\equiv R^{\rm T}\Cal{C}^{-1}R  = \Lambda_0 + [\Lambda_0,\epsilon] - \Lambda_0\,\kappa\,\Lambda_0 + \ldots\,,
\label{app:rotateCinv}
\ee 
where we defined the matrix $\kappa(\theta)$ as
\be 
\kappa(\theta) \equiv R_0^{\rm T}(\delta\theta \cdot \nabla\Cal{C})R_0\,,
\label{app:kappa-def}
\ee
i.e., $\kappa$ is the rotated version of the parameter-dependent perturbation in \Cal{C}.

It is easy to see that the commutator $[\Lambda_0,\epsilon]$ that appears in \eqn{app:rotateCinv} is symmetric, trace-free and has diagonal elements zero. Explicitly, 
\be
[\Lambda_0,\epsilon]_{\alpha\beta} = \left(\lambda_{0\alpha}-\lambda_{0\beta}\right)\epsilon_{\alpha\beta}\,.
\label{app:Lam0eps-comm}
\ee
Requiring $\Lambda$ to be diagonal then gives an expression for the off-diagonal elements of $\epsilon$:
\be
\red{\epsilon_{\alpha\beta} = \frac{\lambda_{0\alpha}\lambda_{0\beta}}{(\lambda_{0\alpha}-\lambda_{0\beta})}\kappa_{\alpha\beta} \,;\quad \alpha\neq\beta}\,,
\label{app:epsilon-value}
\ee
and the eigenvalues of $\Cal{C}^{-1}$ are given by
\be
\lambda_\alpha = \lambda_{0\alpha}\left(1 - \lambda_{0\alpha}\kappa_{\alpha\alpha}\right)\,.
\label{app:lambda}
\ee
These would be independent of $\theta$ at the lowest order provided $\p\kappa_{\alpha\alpha}/\p\theta_i=0$, i.e.,
\be
\left(R_0^{\rm T}\,\nabla\Cal{C}\,R_0\right)_{\alpha\alpha} = 0\,, \quad {\rm or} \quad \kappa_{\alpha\alpha} = 0\,,
\label{app:thetaindep}
\ee 
which makes $\lambda_\alpha\simeq\lambda_{0\alpha}$ at lowest order.

It also follows that, if \eqn{app:thetaindep} holds, then the rotation defined by \eqn{app:epsilon-value} diagonalises $\Cal{C}^{-1}$ and also makes it independent of $\theta$ at the lowest order. Since the contribution to the log-likelihood \eqn{app:loglike} is expected to be dominated by the largest eigenvalues of $\Cal{C}^{-1}$, these conditions only need hold for those eigen-directions $\alpha$. 
In practice, \eqn{app:thetaindep} may be thought of as the requirement $|\lambda_{0\alpha}\kappa_{\alpha\alpha}|\ll1$ (equation~\ref{app:lambda}).

\section{Big table}
\begin{table*}
	\centering
	\begin{tabular}{|c| c| c| c| c| c|} \toprule
	 
	 {\bf Parameters} & $w_p+\xi_{0,2,4}$ & $ \, + (\alpha_{cen},\alpha_{sat})$ & $\, + \rm{VVF}$ & $ \, + \rm{VVF} \, + (\alpha_{cen},\alpha_{sat})$ & ellipsoidal \\ [0.8ex] 
	 \multicolumn{6}{l}{\bf Basic HOD model} \\ \hdashline
	$\log_{10}(M_{\rm cut})$ & $11.71^{+0.11}_{-0.08}$  & $11.79^{+0.17}_{-0.11}$  & $11.63^{+0.08}_{-0.07}$  & $11.93^{+0.07}_{-0.16}$  & $11.84^{+0.24}_{-0.13}$  \\ [0.9ex]
	$\sigma_{\rm M}$ & $0.81^{+0.62}_{-0.37}$  & $1.05^{+0.76}_{-0.45}$  & $0.74^{+0.33}_{-0.37}$  & $1.73^{+0.21}_{-0.52}$  & $1.57^{+0.91}_{-0.5}$  \\ [0.9ex]
	$\log_{10}(M_1)$ & $12.08^{+0.23}_{-0.24}$  & $12.09^{+0.23}_{-0.23}$  & $11.96^{+0.26}_{-0.27}$  & $12.02^{+0.33}_{-0.32}$  & $11.95^{+0.43}_{-0.29}$  \\ [0.9ex]
	$\alpha$ & $0.49^{+0.17}_{-0.13}$  & $0.47^{+0.09}_{-0.1}$  & $0.48^{+0.1}_{-0.08}$  & $0.51^{+0.11}_{-0.06}$  & $0.51^{+0.13}_{-0.07}$  \\ [0.9ex]
	$\kappa$ & $2.47^{+0.34}_{-0.5}$  & $2.36^{+0.38}_{-0.51}$  & $2.67^{+0.21}_{-0.35}$  & $2.26^{+0.4}_{-0.43}$  & $2.38^{+0.28}_{-0.96}$  \\ [0.9ex]
	 \multicolumn{6}{l}{\bf Dynamics and Satellite} \\ \hdashline
	$\gamma_{\rm HV}$ & $0.9^{+0.06}_{-0.06}$  & $0.83^{+0.07}_{-0.07}$  & $0.94^{+0.04}_{-0.05}$  & $0.86^{+0.04}_{-0.05}$  & $0.84^{+0.03}_{-0.06}$  \\ [0.9ex]
	$f_{\rm c}$ & $0.64^{+0.32}_{-0.21}$  & $0.53^{+0.27}_{-0.15}$  & $0.68^{+0.13}_{-0.16}$  & $0.63^{+0.18}_{-0.13}$  & $0.58^{+0.22}_{-0.13}$  \\ [0.9ex]
	$\gamma_{\rm IHV}$ & $1.41^{+0.29}_{-0.3}$  & $1.51^{+0.33}_{-0.26}$  & $1.4^{+0.15}_{-0.16}$  & $1.31^{+0.22}_{-0.11}$  & $1.39^{+0.23}_{-0.2}$  \\ [0.9ex]
	$f_{\rm vir}$ & $2.13^{+0.38}_{-0.44}$  & $2.35^{+0.69}_{-0.42}$  & $2.19^{+0.25}_{-0.21}$  & $2.21^{+0.28}_{-0.36}$  & $2.47^{+0.47}_{-0.13}$  \\ [0.9ex]
	 \multicolumn{6}{l}{\bf Inferred Parameters} \\ \hdashline
	$f_{\rm sat}$ & $0.3 \pm 0.06$  & $0.27 \pm 0.07$  & $0.34 \pm 0.03$  & $0.24 \pm 0.05$  & $0.23 \pm 0.06$  \\ [0.9ex]
	$\bar{n} \, [\mpcoh]^{-3}$ & $0.014 \pm 0.004$  & $0.014 \pm 0.004$  & $0.015 \pm 0.002$  & $0.016 \pm 0.002$  & $0.017 \pm 0.004$  \\ [0.9ex]
	$f\sigma_8(z_{\rm mean})$ & $0.41^{+0.03}_{-0.03}$  & $0.37^{+0.03}_{-0.03}$  & $0.42^{+0.02}_{-0.02}$  & $0.39^{+0.02}_{-0.02}$  & $0.38^{+0.01}_{-0.03}$  \\ [0.9ex]
	 \multicolumn{6}{l}{\bf Assembly Bias Parameters} \\ \hdashline
	$\alpha_{\rm cen}$ &  fixed   & $-0.22^{+0.23}_{-0.26}$  &  fixed   & $-0.71^{+0.29}_{-0.11}$  & $-0.6^{+0.21}_{-0.3}$  \\ [0.9ex]
	$\alpha_{\rm sat}$ &  fixed   & $1.08^{+0.57}_{-0.58}$  &  fixed   & $1.44^{+0.25}_{-0.43}$  & $1.11^{+0.47}_{-0.33}$  \\ [0.9ex] \bottomrule 
	\end{tabular}
 	\caption{this table}
	\label{tab:tt}
\end{table*}
